# Supplementary material for: TRUST: Test-Time Refinement using Uncertainty-Guided SSM Traverses
Source: arXiv:2509.22813 source file (2026-05-07)
Supplement: Supplementary file 1 [file 6_appendix.tex]

\section{Technical Appendices and Supplementary Material}

\subsection{Datasets}

We evaluate the performance and generalization capability of our method across a broad range of \gls{tta} benchmarks, covering both corruption-based robustness and domain generalization. To assess robustness to common corruptions, we evaluate on CIFAR-10-C, CIFAR-100-C, and ImageNet-C \cite{corruption}. These benchmarks apply 15 algorithmically generated corruption types, including noise, blur, weather effects, and digital artifacts, at five severity levels to the clean CIFAR-10, CIFAR-100, and ImageNet datasets. CIFAR-10-C features $10$ coarse-grained classes, while CIFAR-100-C includes $100$ fine-grained categories, offering a more challenging evaluation. ImageNet-C extends these corruptions to the large-scale ImageNet dataset with $1000$ categories, enabling a systematic analysis of model degradation under real-world visual distortions.

To evaluate generalization across domain shifts, we consider PACS \cite{pacs}, ImageNet-Sketch (ImageNet-S) \cite{sketch}, ImageNet-V2 \cite{v2}, and ImageNet-Rendition (ImageNet-R) \cite{R}. PACS comprises four visually distinct domains (Photo, Art Painting, Cartoon, and Sketch), with a shared label space of seven classes. We follow the standard leave-one-domain-out evaluation protocol. ImageNet-S consists of sketch-style representations of ImageNet classes, testing generalization to abstract and minimalist visual forms. ImageNet-V2 offers a cleaner and independently collected test set from the same distribution as ImageNet. ImageNet-R contains $30,000$ images across $200$ ImageNet classes, covering a wide range of artistic renditions including paintings, cartoons, graffiti, embroidery, and video game graphics. It presents a challenging benchmark for style-based distribution shifts. These datasets collectively enable a comprehensive evaluation of a model’s ability to adapt to unseen styles, abstractions, and distributions.

\subsection{Mean Entropy of Different Traversal Permutations.}
As shown in Figure~\ref{main_figure} offline mode, altering the order of spatial traversals in VMamba results in significant variations in mean entropy on ImageNet-C, highlighting the sensitivity of the model’s internal representations to traversal patterns. Higher entropy values indicate less confident predictions, often correlating with reduced robustness under corruption. This underscores the importance of carefully selecting traversal permutations for reliable adaptation.

For a comprehensive view across datasets, we refer to Figure~\ref{heatmap_combined}, which reports entropy values for all permutations across CIFAR10-C, CIFAR100-C, ImageNet-C, ImageNet-S, ImageNet-V2, ImageNet-R, and PACS. Notably, the top-2, top-4, and top-6 traversal permutations with the lowest entropy (highlighted with green cross-hatching) consistently appear across all datasets. This consistency suggests that certain permutations inherently promote more stable and confident representations regardless of the domain, providing a principled basis for selecting effective traversal subsets in our method.

\begin{figure}[h]
    \centering
    \includegraphics[width=\linewidth]{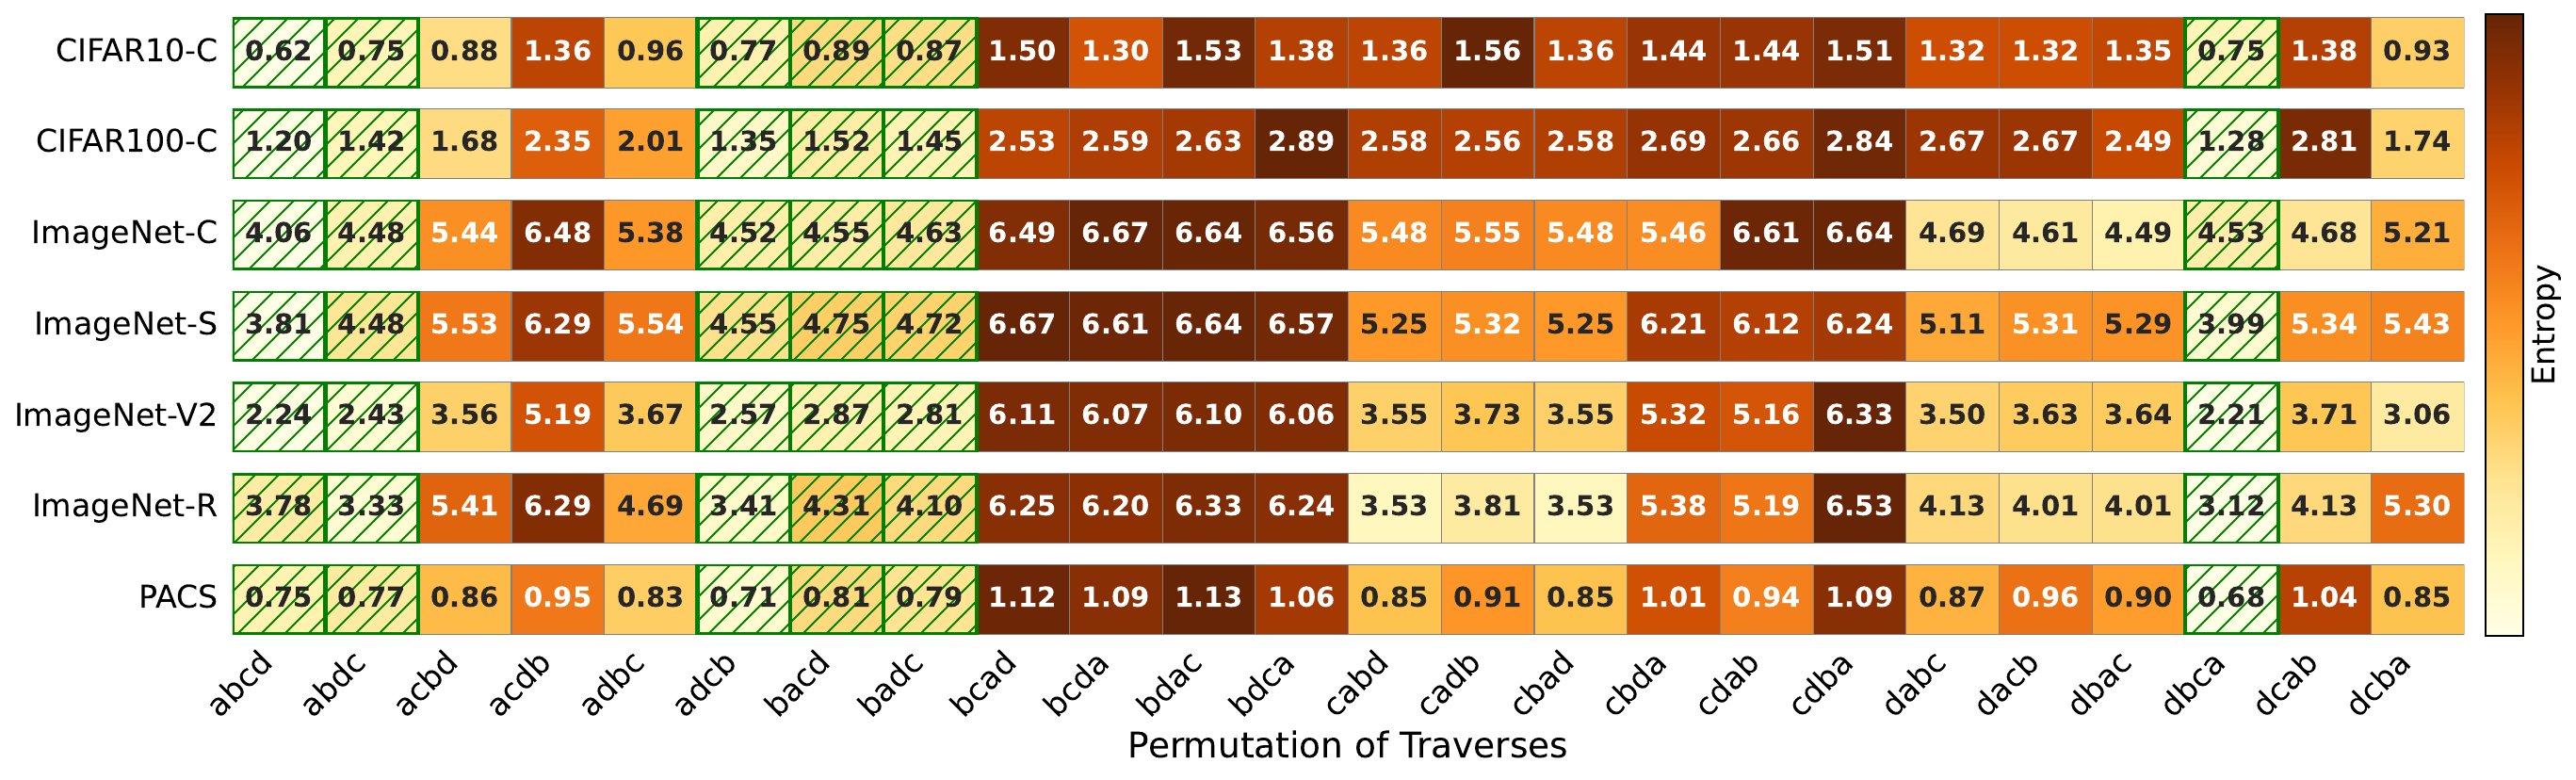}
    \caption{}
    \label{heatmap_combined}
\end{figure}

\subsection{Standard Mode}
\begin{table*}[h]
\setlength\tabcolsep{4pt}
\centering
\resizebox{0.9\textwidth}{!}{
\small
\begin{tabular}{l|l|ccccccc}
\toprule
& \textbf{Method} & CIFAR10-C & CIFAR100-C & ImageNet-C & ImageNet-S & ImageNet-V2 & ImageNet-R & PACS \\
\midrule
\parbox[t]{4mm}{\multirow{7}{*}{\rotatebox[origin=c]{90}{Episodic}}} 
& Source only           & 65.9 & 41.2 & 38.7 & 31.4 & 62.2 & 31.3 & 66.7 \\
& ETA \cite{eta}        & 65.8 & 41.2 & 38.8 & 31.4 & 62.2 & 31.4 & 66.7 \\
& LAME \cite{lame}      & 65.9 & 41.2 & 38.8 & 31.4 & 62.2 & 31.4 & 66.7 \\
& SAR \cite{sar}        & 66.0 & 41.3 & 38.8 & 31.4 & 62.2 & 31.4 & 67.1 \\
\cmidrule{2-9}
& Tent \cite{tent}      & 66.0 & 41.3 & 38.8 & 31.4 & 62.2 & 31.4 & 67.2 \\
& ours naive            & 65.9 & 41.2 & 38.9 & 31.5 & 62.3 & 31.5 & 66.8 \\
& \ccol ours            & \ccol 66.2 & \ccol 41.7 & \ccol 39.9 & \ccol 31.6 & \ccol 62.3 & \ccol 31.5 & \ccol 71.3 \\
\bottomrule
\end{tabular}
}
\caption{Average test-time adaptation performance (accuracy \%) across multiple datasets. For CIFAR10-C, CIFAR100-C, and ImageNet-C, the values represent the mean across all corruption types and severities. For ImageNet-S, ImageNet-V2, ImageNet-R, and PACS, the values correspond to classification accuracy on their respective test sets.}
\label{domain_shift}
\end{table*}

\begin{table*}[h]
\setlength\tabcolsep{4pt}
\centering
\resizebox{0.9\textwidth}{!}{
\small
\begin{tabular}{l|l|ccccccccccccccc|c}
\toprule
& Method & \rotatebox{90}{gaussian noise} & \rotatebox{90}{shot noise} & \rotatebox{90}{impulse noise} & \rotatebox{90}{defocus blur} & \rotatebox{90}{glass blur} & \rotatebox{90}{motion blur} & \rotatebox{90}{zoom blur} & \rotatebox{90}{frost} & \rotatebox{90}{snow} & \rotatebox{90}{fog} & \rotatebox{90}{brightness} & \rotatebox{90}{contrast} & \rotatebox{90}{elastic} & \rotatebox{90}{pixelate} & \rotatebox{90}{jpeg compression} & Mean \\
\midrule
\parbox[t]{4mm}{\multirow{8}{*}{\rotatebox[origin=c]{90}{CIFAR10-C}}} 
& Source only           & 46.8 & 48.4 & 45.0 & 73.5 & 52.6 & 73.0 & 78.7 & 71.8 & 75.8 & 77.3 & 85.7 & 69.6 & 63.7 & 67.9 & 59.0 & 65.9 \\
& ETA \cite{eta}        & 46.6 & 48.3 & 44.8 & 73.5 & 52.6 & 73.0 & 78.6 & 71.4 & 75.7 & 77.2 & 85.7 & 69.6 & 63.7 & 67.9 & 59.0 & 65.8 \\
& LAME \cite{lame}      & 46.7 & 48.3 & 44.8 & 73.5 & 52.6 & 73.0 & 78.6 & 71.8 & 75.8 & 77.2 & 85.7 & 69.6 & 63.7 & 67.9 & 59.0 & 65.9 \\
& SAR \cite{sar}        & 46.8 & 48.4 & 45.0 & 73.6 & 52.7 & 73.1 & 78.7 & 71.8 & 75.9 & 77.3 & 85.7 & 69.7 & 63.9 & 68.0 & 59.1 & 66.0 \\
\cmidrule{2-18}
& Tent \cite{tent}      & 46.7 & 48.4 & 45.0 & 73.7 & 52.7 & 73.1 & 78.8 & 71.9 & 75.9 & 77.4 & 85.7 & 69.7 & 63.8 & 68.1 & 59.0 & 66.0 \\
& Ours naive            & 46.8 & 48.4 & 45.0 & 73.5 & 52.7 & 73.0 & 78.7 & 71.8 & 75.8 & 77.3 & 85.7 & 69.6 & 63.7 & 67.9 & 59.0 & 65.9 \\
& \ccol Ours            & \ccol 47.2 & \ccol 49.5 & \ccol 45.6 & \ccol 73.1 & \ccol 53.1 & \ccol 73.1 & \ccol 78.6 & \ccol 72.1 & \ccol 76.0 & \ccol 77.6 & \ccol 85.6 & \ccol 69.9 & \ccol 63.9 & \ccol 68.2 & \ccol 59.1 & \ccol 66.2 \\
\midrule
\parbox[t]{4mm}{\multirow{8}{*}{\rotatebox[origin=c]{90}{CIFAR100-C}}} 
& Source only           & 21.0 & 22.1 & 18.3 & 50.6 & 27.7 & 51.0 & 56.2 & 45.3 & 50.6 & 52.4 & 65.3 & 43.2 & 39.0 & 41.7 & 33.4 & 41.2 \\
& ETA \cite{eta}        & 21.0 & 22.1 & 18.3 & 50.6 & 27.7 & 51.0 & 56.2 & 45.1 & 50.5 & 52.4 & 65.3 & 43.3 & 39.1 & 41.7 & 33.5 & 41.2 \\
& LAME \cite{lame}      & 21.0 & 22.1 & 18.3 & 50.6 & 27.7 & 51.0 & 56.2 & 45.3 & 50.6 & 52.5 & 65.4 & 43.2 & 39.0 & 41.7 & 33.4 & 41.2 \\
& SAR \cite{sar}        & 21.2 & 22.1 & 18.4 & 50.7 & 27.8 & 51.0 & 56.3 & 45.5 & 50.7 & 52.6 & 65.4 & 43.3 & 39.1 & 41.8 & 33.5 & 41.3 \\
\cmidrule{2-18}
& Tent \cite{tent}      & 21.1 & 22.2 & 18.4 & 50.6 & 27.7 & 51.0 & 56.2 & 45.1 & 50.5 & 52.3 & 65.4 & 43.3 & 39.0 & 41.7 & 33.4 & 41.2 \\
& Ours naive            & 21.1 & 22.2 & 18.4 & 50.6 & 27.7 & 51.0 & 56.2 & 45.1 & 50.5 & 52.3 & 65.4 & 43.3 & 39.0 & 41.7 & 33.4 & 41.2 \\
& \ccol Ours            & \ccol 21.9 & \ccol 23.1 & \ccol 19.1 & \ccol 50.9 & \ccol 28.1 & \ccol 51.4 & \ccol 56.5 & \ccol 46.0 & \ccol 51.2 & \ccol 53.0 & \ccol 65.4 & \ccol 43.6 & \ccol 39.4 & \ccol 42.3 & \ccol 33.8 & \ccol 41.7 \\
\midrule
\parbox[t]{4mm}{\multirow{8}{*}{\rotatebox[origin=c]{90}{ImageNet-C}}} 
& Source only           & 24.3 & 26.1 & 25.1 & 22.2 & 23.2 & 35.4 & 43.2 & 49.3 & 48.4 & 56.9 & 70.0 & 26.8 & 45.1 & 43.7 & 41.4 & 38.7 \\
& ETA \cite{eta}        & 24.4 & 26.2 & 25.1 & 22.3 & 23.2 & 35.5 & 43.3 & 49.4 & 48.5 & 57.0 & 70.1 & 26.9 & 45.1 & 43.7 & 41.5 & 38.8 \\
& LAME \cite{lame}      & 24.3 & 26.1 & 25.1 & 22.2 & 23.2 & 35.4 & 43.2 & 49.3 & 48.4 & 56.9 & 70.0 & 26.8 & 45.1 & 43.7 & 41.4 & 38.8 \\
& SAR \cite{sar}        & 24.4 & 26.2 & 25.2 & 22.3 & 23.3 & 35.3 & 43.3 & 49.4 & 48.4 & 57.0 & 70.1 & 27.3 & 45.2 & 43.8 & 41.5 & 38.9 \\
\cmidrule{2-18}
& Tent \cite{tent}      & 24.4 & 26.3 & 25.2 & 22.3 & 23.3 & 35.3 & 43.3 & 49.4 & 48.4 & 57.0 & 70.1 & 27.3 & 45.2 & 43.8 & 41.5 & 38.9 \\
& Ours naive            & 24.4 & 26.4 & 25.1 & 22.3 & 23.3 & 35.3 & 43.3 & 49.4 & 48.4 & 57.0 & 70.1 & 27.3 & 45.2 & 43.8 & 41.5 & 38.9 \\
& \ccol Ours            & \ccol 25.9 & \ccol 27.7 & \ccol 26.3 & \ccol 24.0 & \ccol 25.0 & \ccol 36.3 & \ccol 44.3 & \ccol 50.1 & \ccol 49.1 & \ccol 57.8 & \ccol 70.8 & \ccol 28.7 & \ccol 46.0 & \ccol 45.4 & \ccol 43.2 & \ccol 39.9 \\
\bottomrule
\end{tabular}
}
\caption{Test-time adaptation performance (accuracy \%) under various corruption types on CIFAR10-C, CIFAR100-C, and ImageNet-C datasets on episodic setting.}
\label{main}
\end{table*}


\subsection{Model Stock}
\begin{figure}[h]
    \centering
    \includegraphics[width=\linewidth]{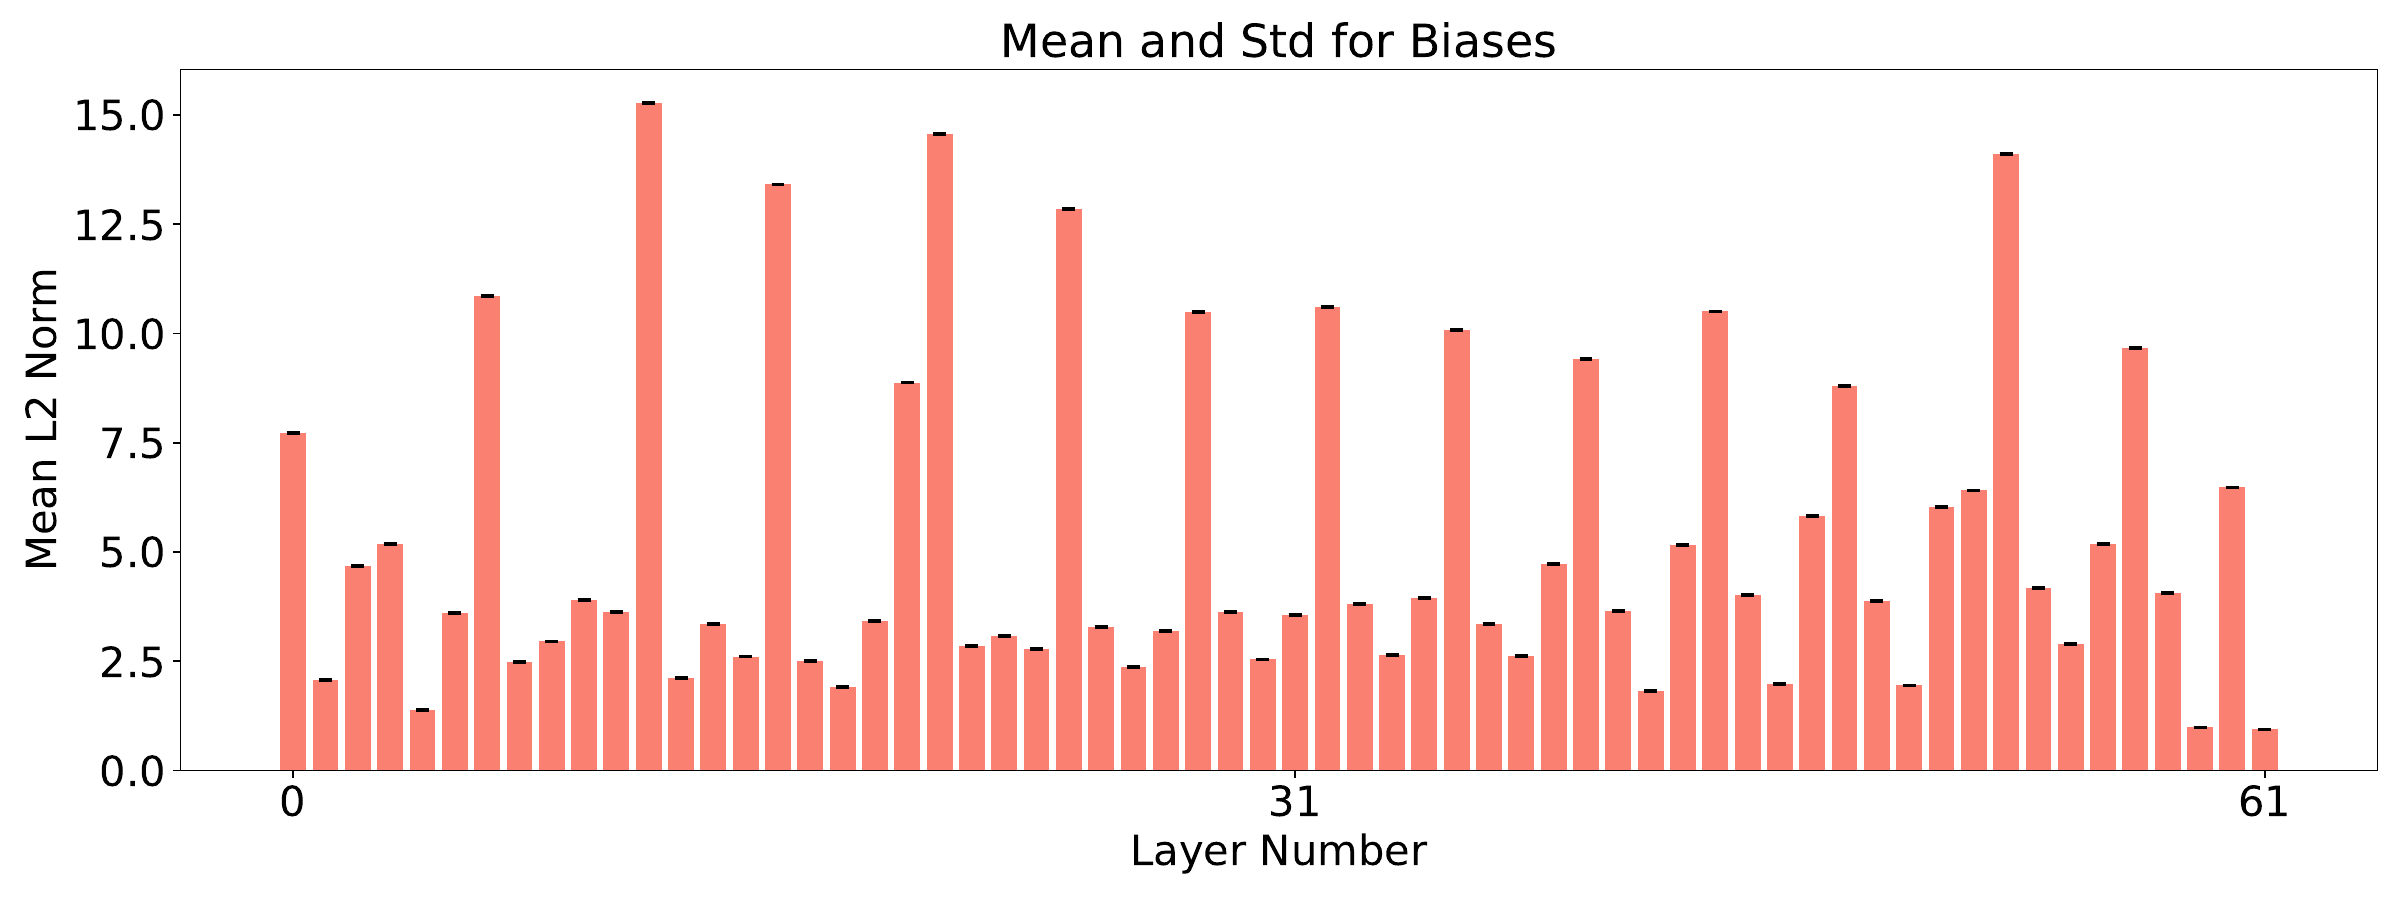}
    \caption{}
    \label{std}
\end{figure}

\begin{figure}[h]
    \centering
    \includegraphics[width=\linewidth]{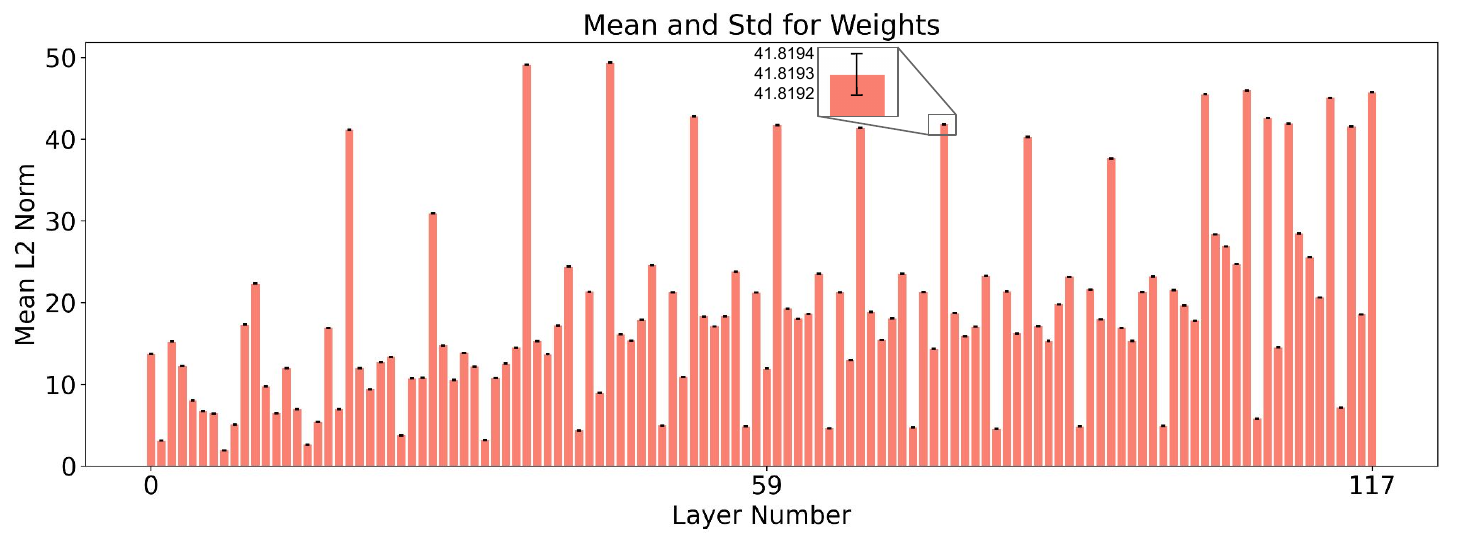}
    \caption{}
    \label{augmentation}
\end{figure}
